# Supplementary material for: TANGO: Training-free Embodied AI Agents for Open-world Tasks
Source: arXiv:2412.10402 source file (2024-12-05)
Supplement: Supplementary file 1 [file X_suppl.tex]

\clearpage
\setcounter{page}{1}
\maketitlesupplementary

\section{Additional Experiments} \label{sec:supp_experiments}

\subsection{Embodied Question Answering}

\setlength{\tabcolsep}{4pt}
\begin{table*}[htbp]
\centering
\begin{tabular}{lccccccccc}
\hline
\noalign{\smallskip}
  &  & \multicolumn{4}{c}{\textbf{Navigation} ($d_T \downarrow$)} & \multicolumn{4}{c}{\textbf{QA} (Top-1 $\uparrow$)} \\ 
\noalign{\smallskip}
\cline{3-10} \noalign{\smallskip}  \textbf{Method} &  Trained & $T_{10}$ & $T_{30}$ & $T_{50}$ & Random & $T_{10}$ & $T_{30}$ & $T_{50}$ & Random \\ 
\noalign{\smallskip}
\hline
\noalign{\smallskip}
PACMAN (BC) \cite{das2018embodied_supp} & \checkmark & 1.19 & 4.25 & 8.12 & N.A. & 48 & 40 & 40 & N.A. \\ 
PACMAN (BC + RF) \cite{das2018embodied_supp} & \checkmark & \textbf{1.05} & 4.22 & 8.13 & N.A. & 50 & 42 & 41 & N.A. \\ 
NMC (BC) \cite{das2019neural_supp} & \checkmark & 1.44 & 4.14 & 8.43 & N.A. & 43 & 41 &  39 & N.A. \\ 
NMC (BC + A3C) \cite{das2019neural_supp} & \checkmark & 1.06 & \textbf{3.72} & 7.94 & N.A. & \textbf{53} &\textbf{46} & 44 & N.A. \\ 
\noalign{\smallskip}
\hline
\noalign{\smallskip}
\approach\ (ours) & \ding{55}  & 3.43 & 4.50 & \textbf{5.26} & \textbf{7.28} & 42 & 40 & 38 & \textbf{37} \\ 
\noalign{\smallskip}
\hline
\noalign{\smallskip}
\rowcolor[gray]{0.9} \approach\ (ours) \begin{footnotesize}+answer constraint\end{footnotesize} & \ding{55} & 3.43 & 4.50 & \textbf{5.26} & \textbf{7.28} & 52 & \textbf{50} & \textbf{48} & \textbf{45} \\ 
\noalign{\smallskip}
\hline
\end{tabular}
\caption{\textbf{MP3D-EQA results.} Comparison of Navigation and QA performance across methods.}
\label{table:mp3d_eqa_results}
\end{table*}
\setlength{\tabcolsep}{1.4pt}

We conducted preliminary experiments with \approach\ on \ac{eqa}, utilizing an older dataset for the task~\cite{das2018embodied_supp}.
In \textsc{\ac{eqa}}, the agent is queried with a natural language question and it must navigate to the target location described in the query and answer accordingly. In the case of the MP3D-EQA dataset~\cite{das2018embodied_supp}, this task is regarded as a classification task aimed at determining the most suitable answer from a set of pre-defined possibilities (i.e., class labels). For this dataset, we have: $24$ colors, $18$ rooms, and $25$ objects with perfect correspondence between train and test set. 
However, \approach\ utilizes a different approach, in which the agent is free to provide an answer independently of predefined target categories, because it is not trained specifically for the task. Nevertheless, Table \ref{table:mp3d_eqa_results} shows that our model yields comparable results against trained methods both in Answer Accuracy (QA) and Distance to goal ($d_{T}$) (row 5), while requiring no training. 
$T_{i}$ is related to $10$, $30$, $50$, random steps away from the target object.
In particular, Neural Modular Controller (NMC) methods~\cite{das2019neural_supp} employ specific navigation policies trained with RL (rows 3-4). 
Furthermore, these models are trained from a predefined list of possible answers. In contrast, our model can provide answers using natural language. 
For example, in episodes where the correct color is described as \textit{``off-white''}, while our agent's output is \textit{``white''}, these instances yield an Answer Accuracy of $0\%$, despite being similar answers. 
Therefore, we evaluated our model with an ``answer constraint'' mechanism in which similar answers were grouped into the same answer. Results show that our method provides the best results among $30$ and $50$ steps away, surpassing by 4\% the best performing method, confirming that \approach\ is able to navigate towards the target object even when it is far from it in the initial position.
%Therefore, we evaluated our method by means of an additional metric, \textit{Answer Similarity}, measuring the embedding similarity between the ground-truth answer and the output of the VQA model. 
%\approach\ results in a $72\%$ similarity among all answers, showcasing the effectiveness of BLIP in generating responses that are similar to the ground-truth ones.
Furthermore, in the ``answered constraint'' scenario, the primary reasons for failure can be attributed to misclassification or the failure of the object detector to detect the object despite its presence (i.e. failure of the ``detect'' module).

%%%% EQA Datset comparison
\subsubsection{EQA Datasets Comparison}
We compared the two primary datasets used in the \ac{eqa} task within embodied environments~\cite{das2018embodied_supp, majumdar2024openeqa_supp}, aiming to discuss a key limitation of these datasets to approach the given task.
As shown in Figure~\ref{img:eqa_dataset_comparison}, the more recent OpenEQA dataset (row 2) lacks certain important features present in the older MP3D-EQA dataset, such as target localization, which is useful for calculating the agent’s path efficiency, as well as a dedicated training set. Conversely, the older dataset lacks open-vocabulary questions and the novel LLM-scoring metric. 
Therefore, we advocate for further enhancement of these datasets to create a comprehensive and well-designed resource for the \ac{eqa} task, where all of these characteristics are present. 
Moreover, it is reasonable to hypothesize that a model excelling in this task would likely perform well in other purely navigational tasks (e.g., ObjNav, Lifelong Navigation) without additional training, given the generalization required to interpret the input question, navigate the environment, and provide an answer.

\begin{figure}[!t]
\begin{center}
\includegraphics[width=0.5\textwidth]{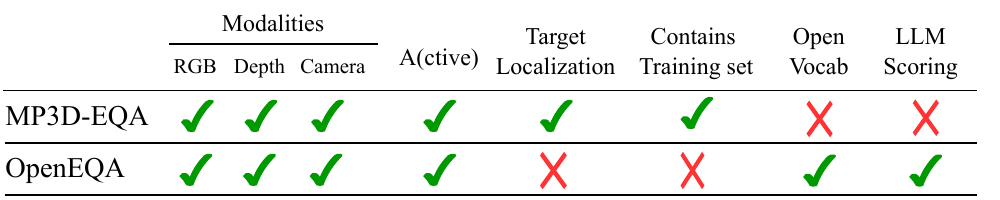}
\caption{\textbf{EQA Datasets comparison.} Dataset comparison between MP3D-EQA~\cite{das2018embodied_supp} and OpenEQA~\cite{majumdar2024openeqa_supp}.}
\label{img:eqa_dataset_comparison}
\end{center}
\end{figure}

\section{Exploration Policy using Memory targets}
\label{sec:supp_exploration_policy}
As described in Section \ref{sec:method}, we extend the exploration policy from \cite{yokoyama2024vlfm_supp} by incorporating a memory mechanism based on a stored feature vector map. At each step, the current RGB observation is processed through a vision-language model (BLIP2 in our implementation~\cite{li2023blip_supp}), updating the current view angle (a triangular-shaped region of pixels on the map) with feature vectors for each pixel. If the navigation target changes, the current value map is updated with a new value map specific to the new target. This new map is calculated by applying cosine similarity between the text or image features of the new target (obtained from the vision-language model) and each pixel's feature vector in the map. Figure \ref{img:exploration_policy} illustrates the following:

\begin{small}
\begin{equation}
    cos \left(\textrm{map}^{val}_{(i,j)}\right) = \frac{\vec{\textrm{map}}^{feat}_{(i,j)} \cdot \vec{\textrm{E}}^{target}}{||\vec{\textrm{map}}^{feat}_{(i,j)}|| \cdot ||\vec{\textrm{E}}^{target}||}  \forall (i,j) \in \textrm{map}^{val}
\label{eq:cosine_similarity}
\end{equation}
\end{small}

where $\vec{\textrm{E}}$ is the embedding vector of the new target (either specified through text or image), $\textrm{map}^{feat}$ is the feature map storing the vector embeddings for each pixel, and $\textrm{map}^{val}$ is the value map used during exploration. Frontiers are retrieved from an obstacle map calculated on the fly~\cite{yokoyama2024vlfm_supp}.

After obtaining the new value map, we assess whether the agent may have already encountered the target object. We sample the highest value in the map, and if it exceeds a defined threshold, we consider the target ``remembered'' and navigate directly to it. If the target object is not found at the expected location, exploration resumes following the standard policy from \cite{yokoyama2024vlfm_supp}. 
Overall, this approach enables more efficient navigation as the model continues to explore, and future work aimed at exploring clustering of high-value regions could be promising.
%As noted in Section \ref{sec:conclusion}, the primary goal of this paper is not to provide an optimal sampling strategy for these points; this can be explored in future work. 

\begin{figure}[!ht]
\begin{center}
\includegraphics[width=.48\textwidth]{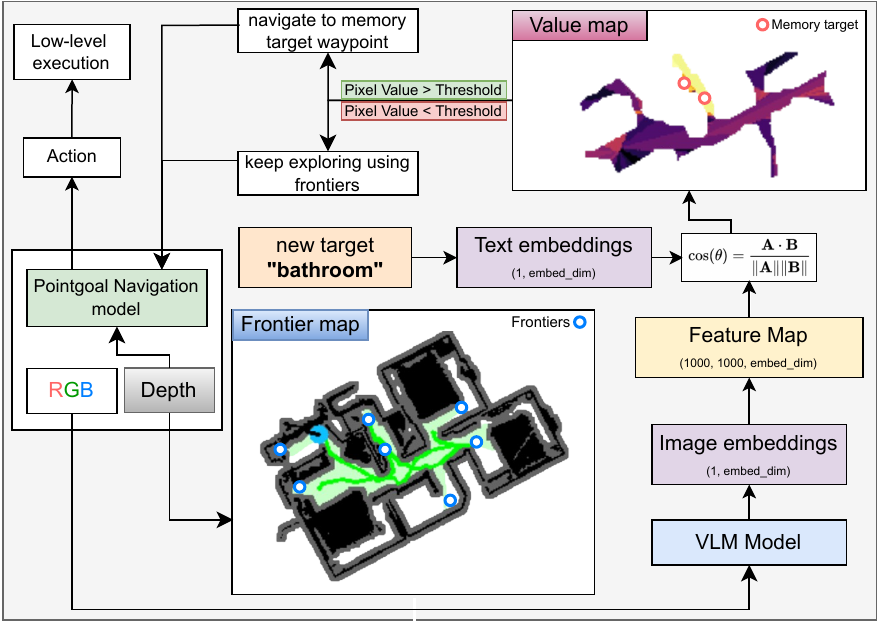}
\end{center}
\caption{\textbf{Exploration Policy.} Illustration of the implemented memory mechanisms in \approach, when a new sequential target is found.}
\label{img:exploration_policy}
\end{figure}

\subsection{Ablation Study}
To evaluate our memory mechanism, we conducted preliminary experiments on multi-target object-goal navigation to identify the optimal threshold, which was then used in the experiments detailed in Section \ref{sec:exp}.
Table~\ref{tab:ablation_memory} presents the results on the Multi-Object Goal Navigation dataset~\cite{wani2020multion_supp}. In this task, similar to ObjectNav, the goal is to navigate to target objects. However, in contrast to ObjectNav, a single episode consists of multiple sequential targets. We evaluated agent performance using three different target types, which are cylindrical objects distinguished by color. The agent is required to locate all targets within a maximum of 2500 steps. If the agent incorrectly calls the ``Found'' action on a target, the entire episode is deemed incorrect. Hence, serving as an effective testbed for evaluating our memory strategy performance.
The ablation study investigates the effect of the memory threshold on the agent's ability to ``remember'' previously encountered objects and navigate to them. Since the value map is normalized between 0 and 1, the memory threshold can take any float value within this range. A threshold of 1 indicates that no memory is used, as it is too high, while a threshold of 0 means that memory is always utilized, potentially leading to incorrect memory-based target selections.
The results show that the optimal memory threshold value is 0.4, as it yields the best overall performance. 
We evaluate the baseline of our approach without memory (row 1) and observe that incorporating memory significantly benefits the agent, improving the success rate by $+5\%$ and path efficiency by $+2\%$ (row 4). 
Additionally, the Progress metric, which tracks the percentage of targets found within a single episode, increases by 4\%. Overall, the memory mechanism helps enhance the agent’s performance.
Notably, thresholds are highly dependent on the normalization applied during value map calculation. For instance, as shown in Table \ref{tab:ablation_memory}, the results peak around threshold values of 0.3 and 0.4. 
As highlighted in Section \ref{sec:conclusion}, further exploration of diverse sampling strategies for high-value region pixels is encouraged.

\setlength{\tabcolsep}{4.4pt}
\begin{table}[!ht]
    \centering
    \begin{tabular}{cccccc}
    \hline
    Memory & Threshold & SR$\uparrow$ & Progress$\uparrow$ & SPL$\uparrow$ & PPL$\uparrow$ \\ \hline
    \ding{55} & \ding{55} & 19 & 39 & 8 & 17 \\ 
    \checkmark &  0.2 & 21 & 39 & 10 & 18 \\ 
    \checkmark &  0.3 & 23 & 42 & 10 & \textbf{20} \\  
    \rowcolor[gray]{0.9} \checkmark &  0.4 & \textbf{24}  & \textbf{43} & \textbf{10} & 19 \\   
    \checkmark &  0.5 & 19 & 40 & 8 & 17 \\ 
    \hline
    \end{tabular}
    \caption{\textbf{\approach\ Ablation Study}. Results on the MultiON dataset~\cite{wani2020multion_supp}, with $3$ sequential targets.}
    \label{tab:ablation_memory}
\end{table}
\setlength{\tabcolsep}{1.4pt}

\section{Failure analysis}

As outlined in Section \ref{sec:exp}, we extracted a significant subsample for the task and manually classified the instances where the model failed. Here we complete the analysis adding the failures in the purely navigational case (see the bottom of Figure \ref{img:failure_analysis_supp}).
For this last case, the majority of failures stem from issues in the navigation and detection modules (9.8\%), rather than planning errors by the \ac{llm} (4.2\%). This discrepancy is due to the fact that navigation tasks inherently involve simpler prompts, such as \textit{``navigate to the chair in the kitchen''}, which clearly specify two distinct targets. These are easier for the \ac{llm} to interpret and sequence effectively.
Furthermore, we observe that the "Timeout" category is more prevalent in Navigation tasks compared to EQA tasks. This is particularly evident in Open-set ObjNav, where targets are often highly ambiguous, making it difficult for the open-set object detector to identify them in simulated 3D environments. Notably, the "Ignored goal object" category accounts for 38\% of failures, significantly higher than the 17.6\% observed in EQA tasks.
In contrast, the "Didn't see target" category remains consistent across both tasks, accounting for approximately 20\% of failures—half the size of the "Ignored goal object" category. This consistency indicates that the navigation policy associated with this category performs reliably for these tasks.
Concerning navigation tasks, we also identified instances where the definition of success threshold distance to the goal appeared overly stringent. Some episodes witnessed the agent halting within 1 meter of the object with the object in view. However, these instances were deemed failures due to the sparse sampling of viewpoints, indicating potential areas for enhancement in the evaluation protocol. 
Specifically, in the case of ObjNav, the same issue was also highlighted in~\cite{raychaudhuri2024mopa_supp}.

\begin{figure}[!ht]
\begin{center}
\includegraphics[width=0.48\textwidth]{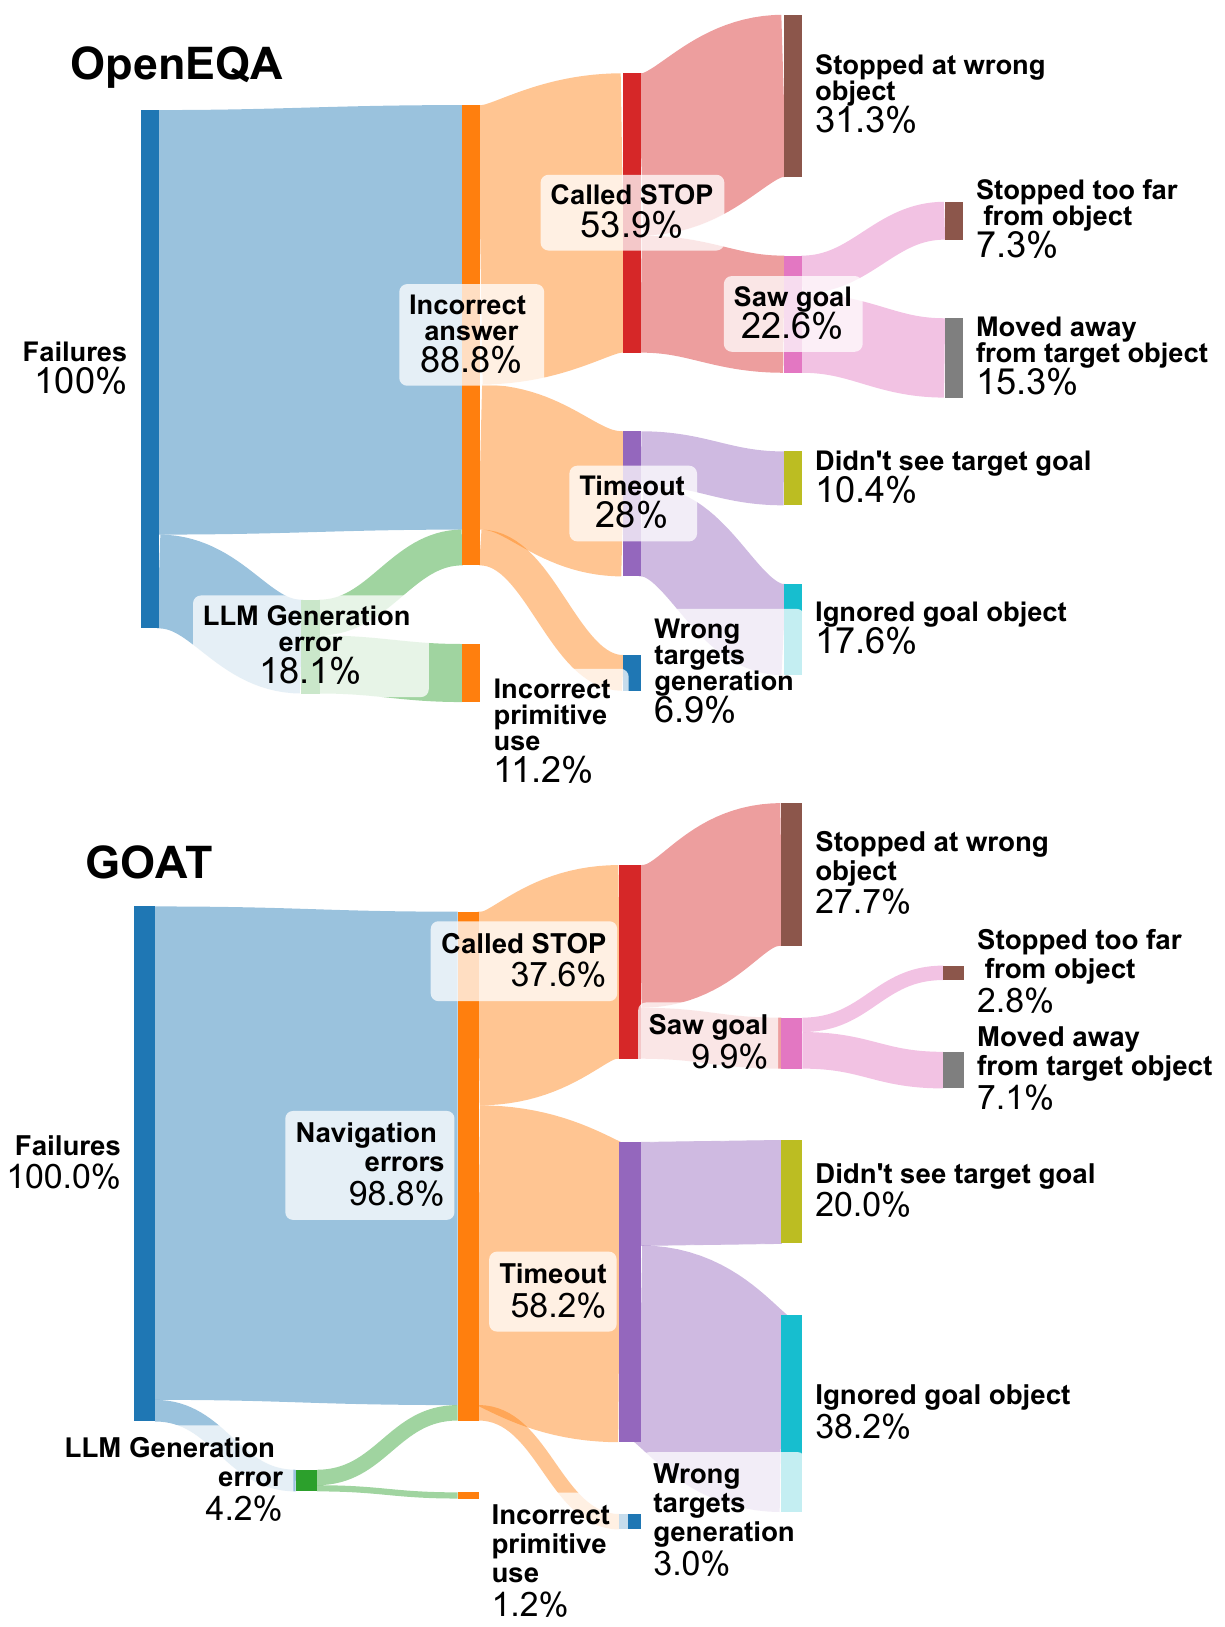}
\caption{\textbf{Failure analysis.} \approach\ failure analysis. (top) OpenEQA failures, (bottom) Goat-Bench, Life Long Multimodal navigation task failures.}
\label{img:failure_analysis_supp}
\end{center}
\end{figure}

%In particular, for \textsc{ObjNav} failure cases exhibit a consistent pattern, primarily attributed to: i) surpassing the maximum step limit, including instances where the agent failed to observe the goal (??\%) and cases where it observed but could not navigate close to it (??\%), and ii) misclassification of the specific target category (??\%), leading the agent to stop at a position away from the goal. 
%In the \textsc{InstanceImageNav} task, failures can primarily be attributed to the MATCH module, which fails to reach the confidence keypoints threshold necessary to correctly classify the target (32\%).
%We considered scores below 3 as failures, i.e. incorrect answers. We observed that the main cause of failure can be attributed to the ``detect'' module (\textit{stopped at wrong object} or \textit{Ignored goal object} in the image). Furthermore, the exploration policy appears to perform well given the targets produced by the \ac{llm}, as it fails in only $\sim10\%$ of the cases (labeled as: \textit{didn't see target goal} in the image). The \ac{llm} generates incorrect pseudo-code around $18\%$ of the time, with $6.9\%$ failures leading to ambiguous or incorrect targets, and $11.2\%$ due to incorrect primitive ordering or usage which instead leads directly to episode failure. 
%Notably, only $11.2\%$ of errors are actually due to the \ac{llm} generating incorrect code, while the remaining is attributable to prompt-related issues.
%A comprehensive failure analysis is provided in the supplementary material.

\section{LLM Prompts.}
\approach\ utilizes \acp{llm} to parse input prompts and generate synthetic pseudocode for task completion. As described in Section \ref{sec:method}, the \ac{llm} is provided with 15 in-context examples spanning various tasks and is tasked with independently composing the appropriate primitives to solve the given task.
The example programs range from simple object-goal navigation (e.g. \textit{``I've lost my laptop, where is it?''}) to multiple \ac{eqa} question-program pairs (e.g. \textit{``Can you tell me if I left the TV on?''}), with the latter being the most challenging to accurately transform into pseudocode, as illustrated in Section \ref{sec:failure_analysis}. The rationale for including diverse tasks is to encourage the \ac{llm} to generalize effectively and learn correct module compositions for specific problems. Therefore, it is the \ac{llm}'s job to understand the current prompt and generate correct pseudocode to tackle the related task.
In particular, in the case it is fed an image as input, it has to first extract the semantic object it represents.
Figure \ref{img:initial_prompt} illustrates the initial prompt structure, including example-program pairs.
Moreover, instructing the \ac{llm} to comment on its own code enhances explainability, which is particularly useful when the model outputs incorrect targets for the task, resulting in a failure.

Figure \ref{img:in_the_wild_example} illustrates an example of \approach\ successfully transforming a target description into a sequence of ordered subtasks. As shown in Table \ref{tab:goat_results}, this transformation enables effective target search within the environment, allowing our approach to achieve the highest results.

\begin{figure}[!ht]
\begin{center}
\includegraphics[width=.48\textwidth]{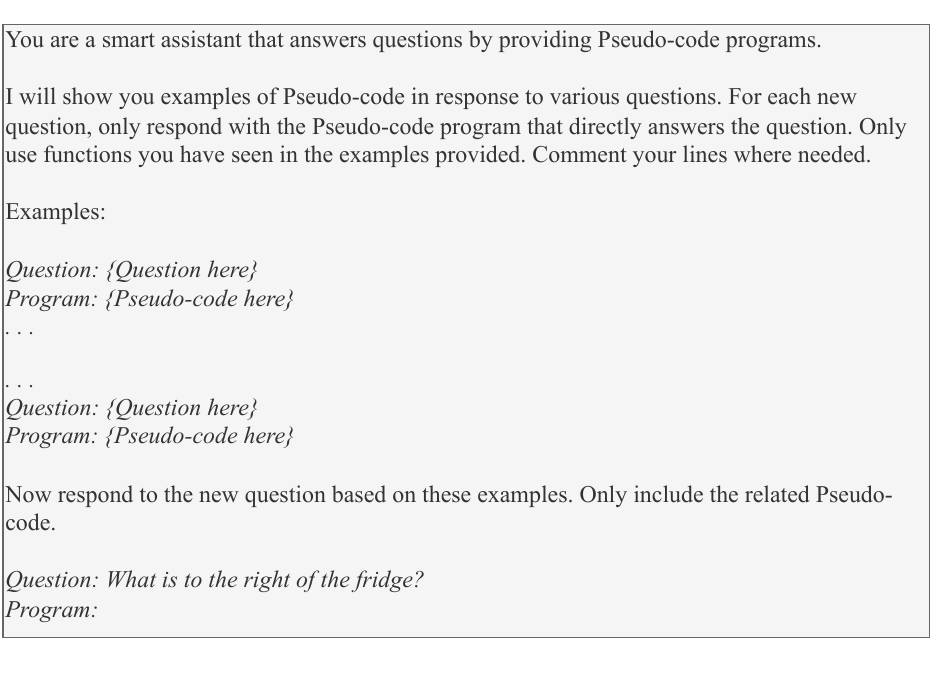}
\caption{\textbf{Initial prompt.} Initial prompt fed to the \ac{llm} to generate the new pseudo-code used in navigation.}
\label{img:initial_prompt}
\end{center}
\end{figure}

\begin{figure}[!ht]
\begin{center}
\includegraphics[width=0.48\textwidth]{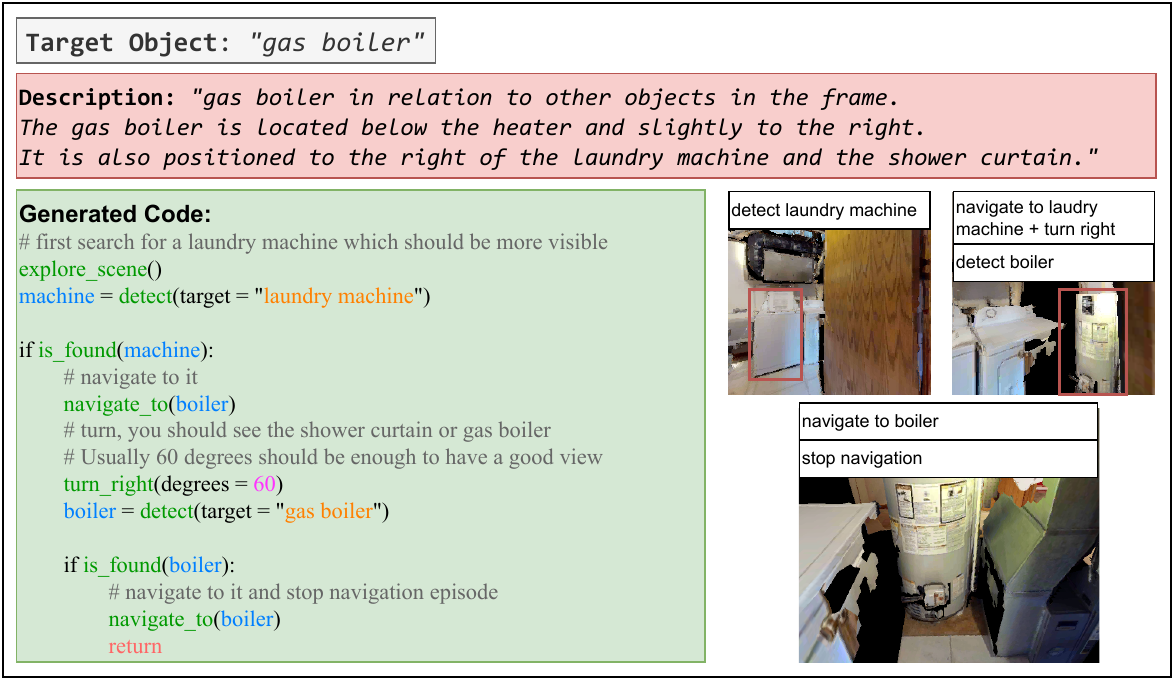}
\caption{\textbf{GOAT subtask example}. The target is \textit{gas boiler} and the agent has to follow the set of primitives generated by the \ac{llm}. Moreover, the comments on the code helps understand the \ac{llm}'s thought process.}
\label{img:in_the_wild_example}
\end{center}
\end{figure}
